# Supplementary material for: Unlearning through Knowledge Overwriting: Reversible Federated Unlearning via Selective Sparse Adapter
Source: arXiv:2502.20709 source file (2025-02-28)
Supplement: Supplementary file 1 [file X_suppl.tex]

\clearpage
\setcounter{page}{1}
\maketitlesupplementary

\section{Algorithm of CLI}
\cref{algo: Critical Layer Identification} outlines the specific process for critical layer identification. The inputs include the original model that needs to executive the unlearning process $\mathcal{M}^r$, the number of local training $E$, the learning rate $\eta$, the number of clients $N$, client data $\mathcal{D}=\cup\left(x_i, y_i\right)_{i=1}^N$, and the number of unlearning layers $K$. The output is a set of unlearning layers $\mathcal{L}^f$. Initially, the server distributes the original model $\mathcal{M}^r$ to all clients (Line 1). Subsequently, each client performs a specified number of local training $E$ iterations on the model using their local data (Lines 2-6). Upon completing local training, the clients upload their models to the server (Line 7). The server then calculates the differences between each client’s model and the globally distributed model layer by layer, based on Equation (12). Each client’s model generates a difference value, and by aggregating these values across different clients, the average difference value for each layer is computed (Line 12). Finally, the difference values for the various layers are ordered in descending order, resulting in a difference list, from which the top $K$ elements are selected to identify the unlearning layers.
\begin{algorithm}[htb]
\caption{Critical Layer Identification}
\label{algo: Critical Layer Identification}
\textbf{Input}: Original model $\mathcal{M}^r$, number of local training $E$, learning rate $\eta$, number of clients $N$, clients data $\mathcal{D}=\cup({x_i},{y_i} )_{i = 1}^N$, number of unlearning layer $K$\\
\textbf{Output}: Unlearning layer $\mathcal{L}^f$
\begin{algorithmic}[1] %[1] enables line numbers
\STATE Server distribute $\mathcal{M}^r$ to all clients
\FOR{ client $n = 1$ \TO $N$}
\FOR{ local epoch $e = 0$ \TO $E-1$}
\STATE $\mathcal{M}_n^r(e+1)=\mathcal{M}_n^r(e)-\eta \nabla F_n(\mathcal{M}_n^r(e),\mathcal{D}_n)$
\ENDFOR
\ENDFOR
\STATE Clients transit local models to the server\\
\FOR{each layer $l = 1$ \TO $L$}
\FOR{client model $\mathcal{M}_n^r(E)$, where $n = 1$ \TO $N$}
\STATE Calculate the $Diff_l^n(p_l^n,{p_l})$ (refer to Eq. 12\\
\ENDFOR
\STATE $Diff_l \gets Aggregate$ ${Diff_l^n(p_l^n,{p_l})}|_{n=1}^N$ (refer to Eq. 13)\\
\ENDFOR
\STATE Sorting $Diff_l$ from large to small and then $LS$ is obtained
\STATE Take the first $K$ elements in $LS$ to obtain the unlearning layer $\mathcal{L}^f$
\STATE \textbf{return} Unlearning layer $\mathcal{L}^f$
\end{algorithmic}
\end{algorithm}

\begin{figure*}[!ht]
	\centering
	\begin{subfigure}[b]{0.33\linewidth}
		\includegraphics[width=\linewidth]{supple/bar_data_fashionmnist_paradigm_client_fnum_5_alpha_1.0.pdf}
		\caption{FashionMNIST.}
		\label{bar_data_fashionmnist_paradigm_client_fnum_5_alpha_1.0}
	\end{subfigure}
	\hfill
	\begin{subfigure}[b]{0.33\linewidth}
		\includegraphics[width=\linewidth]{supple/bar_data_cifar10_paradigm_client_fnum_5_alpha_1.0.pdf}
		\caption{Cifar10.}
		\label{bar_data_cifar10_paradigm_client_fnum_5_alpha_1.0}
	\end{subfigure}
    \hfill
	\begin{subfigure}[b]{0.33\linewidth}
		\includegraphics[width=\linewidth]{supple/bar_data_cifar100_paradigm_client_fnum_5_alpha_1.0.pdf}
		\caption{Cifar100.}
		\label{bar_data_cifar100_paradigm_client_fnum_5_alpha_1.0}
	\end{subfigure}
	\caption{Multi-client unlearning performance.}
	\label{Multi-client unlearning}
\end{figure*}

\begin{figure*}[!ht]
	\centering
	\begin{subfigure}[b]{0.33\linewidth}
		\includegraphics[width=\linewidth]{supple/line_data_fashionmnist_paradigm_class_fnum_1_alpha_1.0.pdf}
		\caption{FashionMNIST.}
		\label{line_data_fashionmnist_paradigm_class_fnum_1_alpha_1.0}
	\end{subfigure}
	\hfill
	\begin{subfigure}[b]{0.33\linewidth}
		\includegraphics[width=\linewidth]{supple/line_data_cifar10_paradigm_class_fnum_1_alpha_1.0.pdf}
		\caption{Cifar10.}
		\label{line_data_cifar10_paradigm_class_fnum_1_alpha_1.0}
	\end{subfigure}
    \hfill
	\begin{subfigure}[b]{0.33\linewidth}
		\includegraphics[width=\linewidth]{supple/line_data_cifar100_paradigm_class_fnum_1_alpha_1.0.pdf}
		\caption{Cifar100.}
		\label{line_data_cifar100_paradigm_class_fnum_1_alpha_1.0}
	\end{subfigure}
	\caption{Class unlearning performance.}
	\label{class unlearning}
\end{figure*}

\section{Experimental hyper-parameters}
The experiment hyper-parameters are shown in \cref{Experimental hyper-parameters}. ``LR" and ``BS" denote learning rate and batch size respectively. ``Sparse Rate" is the dropout ratio of the unlearning layer in the process of sparsification to adapter.

\begin{table}[H]
  \centering
    \begin{tabular}{c|cccc}
    \toprule
          & LR & Optim & BS & Sparse Rate \\
    \midrule
    Fa-MT & 0.005 & SGD   & 64    & 0.1 \\
    Cifar10 & 0.005 & SGD   & 64    & 0.1 \\
    Cifar100 & 0.01  & SGD   & 64    & 0.1 \\
    \bottomrule
    \end{tabular}%
    \caption{Experimental hyper-parameters.}
  \label{Experimental hyper-parameters}%
\end{table}%

\begin{figure*}[!ht]
	\centering
	\begin{subfigure}[b]{0.33\linewidth}
		\includegraphics[width=\linewidth]{supple/line_data_fashionmnist_paradigm_sample_fnum_1_alpha_1.0.pdf}
		\caption{FashionMNIST.}
		\label{line_data_fashionmnist_paradigm_sample_fnum_1_alpha_1.0}
	\end{subfigure}
	\hfill
	\begin{subfigure}[b]{0.33\linewidth}
		\includegraphics[width=\linewidth]{supple/line_data_cifar10_paradigm_sample_fnum_1_alpha_1.0.pdf}
		\caption{Cifar10.}
		\label{line_data_cifar10_paradigm_sample_fnum_1_alpha_1.0}
	\end{subfigure}
    \hfill
	\begin{subfigure}[b]{0.33\linewidth}
		\includegraphics[width=\linewidth]{supple/line_data_cifar100_paradigm_sample_fnum_1_alpha_1.0.pdf}
		\caption{Cifar100.}
		\label{line_data_cifar100_paradigm_sample_fnum_1_alpha_1.0}
	\end{subfigure}
	\caption{Sample unlearning performance.}
	\label{sample unlearning}
\end{figure*}

\begin{figure*}[t]
	\centering
	\begin{subfigure}[b]{0.33\linewidth}
		\includegraphics[width=\linewidth]{supple/resource_fashionmnist.pdf}
		\caption{FashionMNIST.}
		\label{resource_fashionmnist}
	\end{subfigure}
	\hfill
	\begin{subfigure}[b]{0.33\linewidth}
		\includegraphics[width=\linewidth]{supple/resource_cifar10.pdf}
		\caption{Cifar10.}
		\label{resource_cifar10}
	\end{subfigure}
    \hfill
	\begin{subfigure}[b]{0.33\linewidth}
		\includegraphics[width=\linewidth]{supple/resource_cifar100.pdf}
		\caption{Cifar100.}
		\label{resource_cifar100}
	\end{subfigure}
	\caption{Storage sensitivity analysis on various datasets.}
	\label{Storage sensitivity analysis}
\end{figure*}

\section{Results of non-iid distribution}
In the case of non-independent and identically distributed (non-i.i.d.) data on the client, we employ a Dirichlet distribution to partition the dataset and set the hyperparameter to 0.1. The final experimental results are illustrated in \cref{non-iid result}. Compared to the scenario with alpha = 1, nearly all methods exhibited a decline in performance on \textit{RA}. However, the FUSED method maintained a high \textit{RA} and a low \textit{FA}, demonstrating a significant advantage in unlearning effects, with its \textit{ReA} and \textit{MIA} metrics being comparable to those of other methods. Notably, in scenarios involving sample unlearning, the unlearning effect of the FUSED method was on par with that of the retraining, and it even shows a slight advantage in some cases. Moreover, regardless of the dataset or the unlearning scenario, the FUSED method consistently demonstrates a clear superiority in computational resource consumption.

\begin{table*}[htbp]
  \centering
  \resizebox{\textwidth}{!}{
    \begin{tabular}{c|ccccc|cc|ccc}
    \toprule
    \multirow{3}[6]{*}{} & \multicolumn{5}{c|}{\textit{Client Unlearning}} & \multicolumn{2}{c|}{\textit{Class Unlearning}} & \multicolumn{3}{c}{\textit{Sample Unlearning}} \\
\cmidrule{2-11}          & \cellcolor{gray!25}Retrain & \cellcolor{gray!25}Federaser & \cellcolor{gray!25}Exact-Fun & \cellcolor{gray!25}\texttt{FUSED} & \cellcolor{gray!25}EraseClient & \cellcolor{gray!25}Retrain & \cellcolor{gray!25}\texttt{FUSED} &\cellcolor{gray!25}       & \cellcolor{gray!25}Retrain & \cellcolor{gray!25}\texttt{FUSED} \\
\cmidrule{2-11}          & \multicolumn{10}{c}{\textit{FashionMNIST-LeNet}} \\
    \midrule
    \cellcolor{gray!25}\textit{RA($\uparrow$) }   & 0.96  & 0.94  & \underline{0.98}  & \textbf{0.99 } & 0.90  & \textbf{0.99 } & 0.98  & \cellcolor{gray!25}\textit{0A($\uparrow$)  }   & \textbf{1.00 } & \textbf{1.00 } \\
    \cellcolor{gray!25}\textit{FA($\downarrow$)}    & \textbf{0.00 } & \underline{0.01}  & 0.00  & \textbf{0.00 } & 0.01  & \textbf{0.00 } & \textbf{0.00 } & \cellcolor{gray!25}\textit{PS($\uparrow$)  }   & \textbf{1.00 } & \textbf{1.00 } \\
    \cellcolor{gray!25}\textit{ReA($\downarrow$) }  & \textbf{0.87 } & 0.90  & 0.98  & \underline{0.88}  & 0.96  & \textbf{1.00 } & \textbf{1.00 } & \cellcolor{gray!25}\textit{ReA($\downarrow$)}   & \textbf{0.09 } & 0.40  \\
    \cellcolor{gray!25}\textit{MIA($\downarrow$) }  & 0.91  & \underline{0.70}  & 0.90  & 0.82  & \textbf{0.00 } & \textbf{0.95 } & 0.99  & \cellcolor{gray!25}\textit{MIA($\downarrow$)  } & \textbf{0.66 } & 0.99  \\
    \cellcolor{gray!25}\textit{Comp($\downarrow$)}  & 887.04  & 453.77  & 881.74  & \textbf{498.01 } & 1060.44  & 864.44  & \textbf{789.88 } & \cellcolor{gray!25}\textit{Comp($\downarrow$) } & 1000.80  & \textbf{997.55 } \\
    \midrule
          & \multicolumn{10}{c}{\textit{Cifar10-ResNet18}} \\
    \midrule
    \cellcolor{gray!25}\textit{RA($\uparrow$)}     & 0.28  & 0.17  & 0.21  & \textbf{0.45 } & \underline{0.35}  & 0.46  & \textbf{0.57 } & \cellcolor{gray!25}\textit{0A($\uparrow$)}     & 0.72  & \textbf{0.75 } \\
    \cellcolor{gray!25}\textit{FA($\downarrow$) }    & \textbf{0.01 } & 0.20  & 0.13  & \textbf{0.01 } & \underline{0.12}  & 0.00  & \textbf{0.00 } & \cellcolor{gray!25}\textit{PS($\uparrow$) }    & 0.56  & \textbf{0.70 } \\
    \cellcolor{gray!25}\textit{ReA($\downarrow$)}   & 0.70  & \underline{0.41}  & \textbf{0.40 } & 0.55  & 0.45  & 1.00  & \textbf{1.00 } & \cellcolor{gray!25}\textit{ReA($\downarrow$)}   & 0.82  & \textbf{0.75 } \\
    \cellcolor{gray!25}\textit{MIA($\downarrow$)}   & 0.79  & 1.00  & \textbf{0.49 } & 0.82  & \underline{0.75}  & 0.97  & \textbf{0.81 } & \cellcolor{gray!25}\textit{MIA($\downarrow$)}   & \textbf{0.94 } & 0.96  \\
    \cellcolor{gray!25}\textit{Comp($\downarrow$)}  & 1525.13  & 1664.39  & 1583.59  & \textbf{257.66 } & 1801.29  & 580.04  & \textbf{349.79 } & \cellcolor{gray!25}\textit{Comp($\downarrow$)}  & 739.90  & \textbf{533.88 } \\
    \midrule
          & \multicolumn{10}{c}{\textit{Cifar100-ResNet18}} \\
    \midrule
    \cellcolor{gray!25}\textit{RA($\uparrow$)}     & \underline{0.27} & 0.02  & 0.22  & \textbf{0.30 } & 0.25  & \textbf{0.21 } & 0.13  & \cellcolor{gray!25}\textit{0A($\uparrow$)}     & 0.33  & \textbf{0.33 } \\
    \cellcolor{gray!25}\textit{FA($\downarrow$)}    & \underline{0.01}  & 0.02  & \textbf{0.00 } & 0.03  & 0.02  & \textbf{0.00 } & \textbf{0.00 } & \cellcolor{gray!25}\textit{PS($\uparrow$) }    & 0.08  & \textbf{0.50 } \\
    \cellcolor{gray!25}\textit{ReA($\downarrow$)}   & \textbf{0.21 } & 0.21  & 0.26  & \underline{0.22}  & 0.22  & \textbf{1.00 } & \textbf{1.00 } & \cellcolor{gray!25}\textit{ReA($\downarrow$)}   & \textbf{0.00 } & 0.01  \\
    \cellcolor{gray!25}\textit{MIA($\downarrow$) }  & \underline{0.03}  & \textbf{0.00 } & 0.08  & 0.48  & 0.41  & 0.85  & \textbf{0.39 } & \cellcolor{gray!25}\textit{MIA($\downarrow$)}   & \textbf{0.98 } & 1.00  \\
    \cellcolor{gray!25}\textit{Comp($\downarrow$)}  & 1592.70  & 1662.91  & 1683.16  & \textbf{257.42 } & 1918.78  & 789.58  & \textbf{376.82 } & \cellcolor{gray!25}\textit{Comp($\downarrow$)}  & 797.95  & \textbf{526.92 } \\
     \bottomrule
    \end{tabular}}%

  \caption{Expetimental result under non-iid. The bolded numbers represent the best, while the underlined numbers represent the second best.}
  \label{non-iid result}%
\end{table*}%

\section{Experiments of multi-client unlearning}
In the main manuscript, we have validated the scenario of forgetting knowledge from a single client. Furthermore, the proposed method is also effective in scenarios involving the forgetting of knowledge across multiple clients. Therefore, based on an experimental framework with 50 clients, we assume that 50\% of the clients are subjected to Byzantine attacks. The final results are presented in \cref{results of multi-client unlearning}, and the corresponding are shown in \cref{Multi-client unlearning}. The experimental results indicate that \texttt{FUSED}'s unlearning effect is surpassed only by that of Retraining. Compared to other methods, \texttt{FUSED} demonstrates an average improvement of 11.3\% in testing accuracy for the remaining knowledge, while the testing accuracy for the forgotten knowledge is reduced by an average of 8.5\%.

% Table generated by Excel2LaTeX from sheet '附录结果'
\begin{table}[htbp]
  \centering
  \resizebox{\columnwidth}{!}{
    \begin{tabular}{c|c|ccccc}
    \toprule
    \multicolumn{1}{c}{} &       & Retrain & Federaser & E-F & \texttt{FUSED} & E-C \\
    \midrule
    \multirow{2}[2]{*}{Fa-MT} & RA & \textbf{0.99}  & 0.96  & \underline{0.98}  & \underline{0.98}  & \underline{0.98} \\
          & FA & \textbf{0}     & 0     & 0     & \textbf{0}     & 0 \\
    \midrule
    \multirow{2}[2]{*}{Cifar10} & RA & \textbf{0.65}  & \underline{0.6}   & 0.59  & 0.59  & 0.53 \\
          & FA & \textbf{0.05}  & 0.05  & 0.05  & \textbf{0.05}  & 0.05 \\
    \midrule
    \multirow{2}[2]{*}{Cifar100} & RA & \textbf{0.32}  & 0.18  & \underline{0.28}  & \underline{0.28}  & 0.26 \\
          & FA & \textbf{0.01}  & 0.01  & 0.01  & \textbf{0.01}  & 0.01 \\
    \bottomrule
    \end{tabular}}%
    \caption{The experimental results of multi-client unlearning.}
  \label{results of multi-client unlearning}%
\end{table}%

\section{Class unlearning}
In class unlearning, we assume that a specific class needs to be forgotten. Since most existing research on FU focuses on client unlearning, we mainly compare our method with Retraining (illustrated in \cref{class unlearning}). As shown in the figures, both methods can almost completely forget the targeted class. Although Retraining still holds an advantage in remembered performance, the results of both methods are quite similar.

\section{Sample unlearning}
We test sample unlearning based on backdoor attacks. Specifically, we randomly select 10\% of data from any client, setting the last pixel value of each channel to 255 and modifying its label to 0. By mixing modified data with other data and conducting federated training, we obtain a model such that when a sample with a last pixel value of 255 is detected, its predicted label is always 0, regardless of its true label. We validated our approach only on the FashionMNIST, Cifar10, and Cifar100 datasets, with results shown in \cref{sample unlearning}. We evaluate the effectiveness of unlearning using the precision of samples predicted as 0 (precision) and the accuracy of samples with true labels of 0 (Acc\_zero). The two indicators remain comparable between Retraining and \texttt{FUSED}. In terms of precision, the advantages of \texttt{FUSED} are particularly pronounced on the FashionMNIST dataset. For the Cifar10 dataset, the performance of both methods is comparable; however, in the Cifar100 dataset, \texttt{FUSED} outperforms Retraining by approximately 20\%. These observations indicate that, in the sample unlearning scenario, Retraining does not exhibit a clear advantage over \texttt{FUSED}.

\section{Storage sensitivity analysis}
In the process of calculating unlearning cost, we observed that the Federaser and EraseClient require saving all client models and the global model for each iteration. This necessitates a substantial amount of storage resources, which increases significantly with the number of clients and the number of iterations. To illustrate this, we compared the storage resource consumption of the Federaser, EraseClient, and FUSED under different client and iteration scenarios, as shown in \cref{Storage sensitivity analysis}. The results indicate that, for all datasets, the storage resource consumption of Federaser and EraseClient exhibits a linear relationship with the number of iterations, a trend that becomes more pronounced as the number of clients increases. In contrast, FUSED does not exhibit an increase in storage resource overhead as the number of iterations increases, and the resource consumption burden resulting from the increasing number of clients is relatively small.
